# Supplementary material for: Expressive and Generalizable Low-rank Adaptation for Large Models via Slow Cascaded Learning
Source: arXiv:2407.01491 source file (2024-07-01)
Supplement: Supplementary file 1 [file appendix.tex]

\appendix

\section{Appendix / supplemental material}

% \subsection{Pseudo Code for \ourmethod}
